# Supplementary material for: MerGen: Micro-electrode recording synthesis using a generative data-driven approach
Source: arXiv:2503.16928 source file (2025-03-21)
Supplement: Supplementary file 1 [file 08_Appendices.tex]

\appendices
\section{VQ-VAE Architecture}

\section{Transformer Architecture}
